# Supplementary material for: From Examples to Rules: Neural Guided Rule Synthesis for Information Extraction
Source: arXiv:2202.00475 source file (2022-01-16)
Supplement: Supplementary file 1 [file appendix.tex]

\section{Transitions}
\label{sec:appendix_transitions}

The possible expansions are \todo{add}.

\section{Hyperparameters and Training Procedure}
\label{sec:hyperparameters}

We trained in three stages, in a similar approach to curriculum learning \cite{stretcu2019curriculum}. In the first stage we train for 3 epochs only on sentences with less than $20$ tokens in total and less than $5$ highlighted tokens (easy difficulty). In the second stage, we continue from the previous stage checkpoint and train for an additional 2 epochs on sentences with less than $30$ tokens in total and less than $7$ highlighted tokens (medium difficulty). Finally, we train for one epoch on our complete dataset. We used the same hyperparameters across all stages, listed in Table \ref{tab:hyperparam}. We did not fine-tune our hyperparameters.

\begin{table}[]
\begin{tabular}{l|l}
Batch Size & 256              \\
Epochs     & 3,2,1            \\
Scheduler  & triangular2 \cite{smith2015nomore} \\
Learning rate (start) & 6e-6 \\
Learning rate (end)   & 3e-5 \\
Stages     & 3 \\
Seed       & 1
\end{tabular}
\caption{The hyperparameters we used in training.}
\label{tab:hyperparam}
\end{table}

\section{Computational environment}
We list our training environment in Table \ref{tab:training_environment}.
\begin{table}[]
\begin{tabular}{l|l}
GPU & RTX Titan, 24GB \\
CPU & \begin{tabular}[c]{@{}l@{}}AMD Ryzen Threadripper 3960X \\ 24-Core Processor\end{tabular} \\
RAM & 126 GB
\end{tabular}
\caption{Our training environment}
\label{tab:training_environment}
\end{table}

\section{Random Clusters}
\label{sec:appendix_random_examples}
In Table \ref{tab:random_examples} we list 7 random clusters from the train partition of TACRED, together with their synthesized rule (if any). This complements the examples from Table \ref{tab:examples}.

\begin{table*}
    \begin{tabular}{l}
        \toprule
        \textbf{Spans in cluster:} \\
        medical advisor \\
        shareholders approve takeover by Unicredit Capitalia Chairman \\
        \textbf{Synthesized rule:} \\
        $\cdot$ \\
        \midrule
        \textbf{Spans in cluster:} \\
        – If you follow the thinking that \\
        \textbf{Synthesized rule:} \\
        \text{[lemma="–"] [tag=IN] [tag=PRP] [tag=VBP] [lemma=the] [tag=NN] [tag=WDT]} \\
        \midrule
        \textbf{Spans in cluster:} \\
        was convicted of assault , weapons possession and \\
        , for assault , weapon possession and \\
        \textbf{Synthesized rule:} \\
        $\cdot$ \\
        \midrule
        
        \textbf{Spans in cluster:} \\
        died of a \\
        \textbf{Synthesized rule:} \\
        \text{[lemma=die] [tag=IN] [tag=DT]} \\
        \midrule
        \textbf{Spans in cluster:} \\
        's \\
        \textbf{Synthesized rule:} \\
        \text{[word="\'s"]} \\
        \midrule
        \textbf{Spans in cluster:} \\
        -LRB- LeT -RRB- from \\
        , a 25-year-old from \\
        , the 87 - year-old  \\ 
        \textbf{Synthesized rule:} \\
        $\cdot$ \\
        \midrule \\
        \textbf{Spans in cluster:} \\
        model Adam Senn -- and she introduced \\
        promoted Managing Editor $\dots$ <15 words> $\dots$ executives  John Daniszewski , \\
        spokeswoman confirmed that Heidi and \\
        \textbf{Synthesized rule:} \\
        $\cdot$ \\
        \bottomrule
        
    \end{tabular}
    \caption{Random clusters together with their synthesized rule (if any). The clusters are from the train partition of TACRED \cite{zhang2017tacred}}
    \label{tab:random_examples}
\end{table*}

% \section{Static costs}

% \begin{table}
%   \scalebox{0.8}{
%     \input{tables/ast_costs}
%   }

%     \caption{The costs that we use in our static weights approach}
%   \label{tab:ast_costs}
% %  \vspace{-4mm}
% \end{table}
